# Supplementary material for: Efficient Click-Through Rate Prediction for Developing Countries via Tabular Learning
Source: arXiv:2104.07553 source file (2021-04-15)
Supplement: Supplementary file 1 [file appendix.tex]

\appendix
\section{Appendix}
You may include other additional sections here.
